# Supplementary material for: Gradient Perturbation is Underrated for Differentially Private Convex Optimization
Source: arXiv:1911.11363 source file (2020-10-26)
Supplement: Supplementary file 1 [file appendix.tex]

\begin{appendices}
\section{Proofs Related to DP-GD and DP-SGD}
\label{apd:dp-sgd}

\begin{proof}[Proof of Theorem~\ref{thm:DP-GD-C}]

\end{proof}

\begin{proof}[Proof of Theorem~\ref{thm:DP-SGD-SC-non-smooth} and~\ref{thm:DP-SGD-SC-non-smooth-n}]

We start by giving a useful lemma.
\begin{lemma}
\label{lma:convergence}
Choose $\eta_{t}=\frac{1}{\nu t}$, the expected solution error of $\vx_{t}$ in Algorithm~\ref{alg:DP-SGD} for any $t>1$ satisfies 
\[\mathbb{E}[\norm{\vx_{t}-\vx_{*}}^{2}]\leq\frac{2L^{2}\left(1+p\sigma^{2}\right)}{t\nu^{2}},\]
\end{lemma}

\begin{proof}[Proof of Lemma~\ref{lma:convergence}]

\end{proof}

It's easy to check that Eq~\ref{eq:lma1-2} holds for arbitrary $\vx$ rather than $\vx_{*}$. Rearrange Eq~\ref{eq:lma1-2} and take expectation, we have
\begin{equation}
\begin{aligned}
\label{eq:thm3-1}
\mathbb{E}[\idot{\vx_{t}-\vx,\nabla F\left(\vx_{t}\right)}]\leq\frac{\mathbb{E}[\norm{\vx_{t}-\vx}^{2}]-\mathbb{E}[\norm{\vx_{t+1}-\vx}^{2}]}{2\eta_{t}} + \frac{\eta_{t}L^{2}\left(1+p\sigma^{2}\right)}{2}.
%\mathbb{E}_{\vz_{t},i_{t}}\norm{\vx_{t+1}-\vx_{*}}^{2}\leq\norm{\vx_{t}-\vx_{*}}^{2}-+\eta_{t}^{2}L^{2}\left(1+p\sigma^{2}\right).
\end{aligned}
\end{equation}

Let $k$ be arbitrarily chosen from $\{1,\ldots,\lfloor T/2 \rfloor\}$. Summing over the last $k+1$ iterations and use convexity to lower bound $\idot{\vx_{t}-\vx,\nabla F\left(\vx_{t}\right)}$ by $F\left(\vx_{t}\right)-F\left(\vx\right)$,

\begin{equation}
\begin{aligned}
\label{eq:thm3-2}
\sum_{t=T-k}^{T}\mathbb{E}[F\left(\vx_{t}\right)-F\left(\vx\right)]&\leq \frac{\mathbb{E}[\norm{\vx_{T-k}-\vx}^{2}]}{2\eta_{T-k}}+\frac{1}{2}\sum_{t=T-k+1}^{T}\mathbb{E}[\norm{\vx_{t}-\vx}^{2}]\left(\frac{1}{n_{t}}-\frac{1}{n_{t-1
}}\right) \\
&-\frac{\mathbb{E}[\norm{\vx_{T+1}-\vx}^{2}]}{2\eta_{T}}+\frac{L^{2}\left(1+p\sigma^{2}\right)}{2}\sum_{t=T-k}^{T}\eta_{t}.
%\mathbb{E}_{\vz_{t},i_{t}}\norm{\vx_{t+1}-\vx_{*}}^{2}\leq\norm{\vx_{t}-\vx_{*}}^{2}-+\eta_{t}^{2}L^{2}\left(1+p\sigma^{2}\right).
\end{aligned}
\end{equation}

Substitute $\eta_{t}=\frac{1}{\nu t}$ and follow the idea in \cite{shamir2013stochastic} by choosing $\vx=\vx_{T-k}$, we arrive at

\begin{equation}
\begin{aligned}
\label{eq:thm3-3}
\sum_{t=T-k}^{T}\mathbb{E}[F\left(\vx_{t}\right)-F\left(\vx_{T-k}\right)]&\leq \frac{\nu}{2}\sum_{t=T-k+1}^{T}\mathbb{E}[\norm{\vx_{t}-\vx_{T-k}}^{2}] 
+\frac{L^{2}\left(1+p\sigma^{2}\right)}{2\nu}\sum_{t=T-k}^{T}\frac{1}{t}.
%\mathbb{E}_{\vz_{t},i_{t}}\norm{\vx_{t+1}-\vx_{*}}^{2}\leq\norm{\vx_{t}-\vx_{*}}^{2}-+\eta_{t}^{2}L^{2}\left(1+p\sigma^{2}\right).
\end{aligned}
\end{equation}

Now we bound $\mathbb{E}[\norm{\vx_{t}-\vx_{T-k}}^{2}]$ for $t\geq T-k$, 

\begin{equation}
\begin{aligned}
\label{eq:thm3-4}
\mathbb{E}[\norm{\vx_{t}-\vx_{T-k}}^{2}] &\leq 2\mathbb{E}[\norm{\vx_{t}-\vx_{*}}^{2}]+2\mathbb{E}[\norm{\vx_{T-k}-\vx_{*}}^{2}] \\
&\leq \frac{4L^{2}\left(1+p\sigma^{2}\right)}{\nu^{2}}\left(\frac{1}{t}+\frac{1}{T-k}\right) \leq \frac{8L^{2}\left(1+p\sigma^{2}\right)}{\nu^{2}}\left(\frac{1}{T-k}\right) \\
&\leq \frac{16L^{2}\left(1+p\sigma^{2}\right)}{T\nu^{2}}.
\end{aligned}
\end{equation}

%Eq~\ref{eq:thm3-4} implies the parameters change slowly in the latter iterations.

Substitute Eq~\ref{eq:thm3-4} into Eq~\ref{eq:thm3-3},
\begin{equation}
\begin{aligned}
\label{eq:thm3-5}
\sum_{t=T-k}^{T}\mathbb{E}[F\left(\vx_{t}\right)-F\left(\vx_{T-k}\right)]&\leq \frac{8kL^{2}\left(1+p\sigma^{2}\right)}{T\nu}+\frac{L^{2}\left(1+p\sigma^{2}\right)}{2\nu}\sum_{t=T-k}^{T}\frac{1}{t}.
%\mathbb{E}_{\vz_{t},i_{t}}\norm{\vx_{t+1}-\vx_{*}}^{2}\leq\norm{\vx_{t}-\vx_{*}}^{2}-+\eta_{t}^{2}L^{2}\left(1+p\sigma^{2}\right).
\end{aligned}
\end{equation}

Let $S_{k}=\frac{1}{k+1}\sum_{t=T-k}^{T}\mathbb{E}[F\left(\vx_{t}\right)]$ be the averaged expected values of the last $k+1$ iterations. We are interested in $S_{0}-F\left(\vx_{*}\right)=\mathbb{E}[F\left(\vx_{T}\right)]-F\left(\vx_{*}\right)$. Now we derive an inequality between $S_{k}$ and $S_{k-1}$. By definition, 

\begin{equation}
\begin{aligned}
\label{eq:thm3-6}
kS_{k-1}=\left(k+1\right)S_{k} - \mathbb{E}[\vx_{T-k}].
\end{aligned}
\end{equation}

Rearrange Eq~\ref{eq:thm3-5} to upper bound $-\mathbb{E}[\vx_{T-k}]$,
\begin{equation}
\begin{aligned}
\label{eq:thm3-7}
S_{k-1}&=\frac{k+1}{k}S_{k} - \frac{\mathbb{E}[\vx_{T-k}]}{k} \\
&\leq \frac{k+1}{k}S_{k}  - \frac{S_{k}}{k} + \frac{8L^{2}\left(1+p\sigma^{2}\right)}{\left(k+1\right)T\nu}+\frac{L^{2}\left(1+p\sigma^{2}\right)}{2k\left(k+1\right)\nu}\sum_{t=T-k}^{T}\frac{1}{t} \\
&\leq S_{k} + \frac{L^{2}\left(1+p\sigma^{2}\right)}{2\nu}\left(\frac{16}{kT}+\frac{1}{k\left(k+1\right)}\sum_{t=T-k}^{T}\frac{1}{t}\right).
\end{aligned}
\end{equation}

Summing over $k=1,\ldots,k=\lfloor T/2 \rfloor$, 
\begin{equation}
\begin{aligned}
\label{eq:thm3-8}
S_{0}\leq S_{\lfloor T/2 \rfloor} + \frac{L^{2}\left(1+p\sigma^{2}\right)}{2\nu}\left(\sum_{k=1}^{\lfloor T/2 \rfloor}\frac{16}{kT}+\sum_{k=1}^{\lfloor T/2 \rfloor}\sum_{t=T-k}^{T}\frac{1}{k\left(k+1\right)t}\right).
\end{aligned}
\end{equation}
%and use Lemma~\ref{lma:convergence} to upper bound $\mathbb{E}[\norm{\vx_{t}-\vx_{*}}^{2}]$
Now we bound $S_{\lfloor T/2 \rfloor}-F(\vx_{*})$. Choose $\vx=\vx_{*}$ and $\eta_{t}=\frac{1}{t\nu}$ in Eq~\ref{eq:thm3-2} ,
\begin{equation}
\begin{aligned}
\label{eq:thm3-9}
\sum_{t=\lceil T/2 \rceil}^{T}\mathbb{E}[F\left(\vx_{t}\right)-F\left(\vx_{*}\right)]&= \frac{\nu\lceil T/2 \rceil\mathbb{E}[\norm{\vx_{\lceil T/2 \rceil}-\vx_{*}}^{2}]}{2}+\frac{\nu}{2}\sum_{t=\lceil T/2 \rceil+1}^{T}\mathbb{E}[\norm{\vx_{t}-\vx_{*}}^{2}] \\
&+\frac{L^{2}\left(1+p\sigma^{2}\right)}{2}\sum_{t=\lceil T/2 \rceil}^{T}\eta_{t}\\
&\leq \frac{L^{2}(1+p\sigma^{2})}{\nu}(1+\sum_{t=\lceil T/2 \rceil+1}^{T}\frac{1}{t} + \sum_{t=\lceil T/2 \rceil}^{T}\frac{1}{2t})\\
&\leq \frac{L^{2}(1+p\sigma^{2})}{\nu}(1 + \frac{3}{2}\sum_{t=\lceil T/2 \rceil}^{T}\frac{1}{t}) \\
&\leq \frac{4L^{2}(1+p\sigma^{2})}{\nu}.
\end{aligned}
\end{equation}

The second inequality uses Lemma~\ref{lma:convergence}. The last inequality holds because the fact that $\sum_{t=\lceil T/2 \rceil}^{T}\frac{1}{t}\leq\log(2)$. Dividing Eq~\ref{eq:thm3-9} by $\lceil T/2 \rceil$, 
\begin{equation}
\begin{aligned}
\label{eq:thm3-10}
S_{\lfloor T/2 \rfloor}-F(\vx_{*})\leq \frac{8L^{2}(1+p\sigma^{2})}{T\nu}.
\end{aligned}
\end{equation}

We have $\sum_{k=1}^{\lfloor T/2 \rfloor}\frac{16}{kT}\leq \frac{16(1+log(T))}{T}$ because it is harmonic sequence. Lastly,
\begin{equation}
\begin{aligned}
\label{eq:thm3-11}
\sum_{k=1}^{\lfloor T/2 \rfloor}\sum_{t=T-k}^{T}\frac{1}{k\left(k+1\right)t}& \leq \sum_{k=1}^{\lfloor T/2 \rfloor} \frac{\log(2)}{k(k+1)} \\
&\leq \sum_{k=1}^{\lfloor T/2 \rfloor} \frac{\log(2)}{k^{2}} \leq 2\log(2).
\end{aligned}
\end{equation}

Plugging these bounds into Eq~\ref{eq:thm3-8}, we have
\begin{equation}
\begin{aligned}
\label{eq:thm3-12}
S_{0}-F(\vx_{*})=\mathcal{O}\left(\frac{(1+p\sigma^{2})L^{2}\log(T)}{T\nu}\right).
\end{aligned}
\end{equation}

Choose $\sigma^{2}=\Theta\left(\frac{Tlog\left(1/\delta\right)}{n^{2}\epsilon^{2}}\right)$ to guarantee $(\epsilon,\delta)$-DP. Set $T=n^{2}\epsilon^{2}$, we have
\begin{equation}
\begin{aligned}
\label{eq:thm3-13}
S_{0}-F(\vx_{*})=\mathcal{O}\left(\frac{pL^{2}\log(n)log\left(1/\delta\right)}{n^{2}\epsilon^{2}\nu}\right).
\end{aligned}
\end{equation}

Set $T= \frac{n\epsilon}{\sqrt{p}}$ and assume $p<n^{2}$, we have
\begin{equation}
\begin{aligned}
\label{eq:thm3-14}
S_{0}-F(\vx_{*})=\mathcal{O}\left(\frac{\sqrt{p}L^{2}\log(n)}{n\epsilon\nu}\right).
\end{aligned}
\end{equation}

\end{proof}

\section{Detailed description on benchmark datasets}
\label{apd:exp}
\begin{table} [h]
\caption{Detailed description of seven real world datasets.}
\centering
\begin{TAB}(r)[0.5pt]{|c|c|c|c|c|c|c|c|}{|c|c|c|c|}
\label{tbl:7-datasets}
dataset						&Adult &KDDCup99		& MNIST		& Covertype & Gisette & Real-sim & RCV1	\\		
\# records				    & 45220    &70000			& 65000   	&581012				& 6000					&72309			&50000  				\\	
\# features					&	104		&	114				&	784					&	54					& 5000			&20958			&47236				\\
\# classes					&2				&2					&10			&7			&2		&2	&2 \\
\end{TAB}
\end{table}

\section{Comparison between Average and Minimum Curvatures on Different dataset}
\label{apd:comparison_curs}

In this section we plot the average and minimum curvatures in Figure~\ref{fig:apd_curs} for another dataset KDDCup99. The objective function is still regularized logistic regression.

\begin{figure}
  \makebox[\textwidth][c]{\includegraphics[width=0.5\linewidth]{imgs/cur_kddcup.pdf}}%
  \caption{Curvatures of regularized logistic regression on KDDCup99 dataset over training. Dot symbol represents average curvature and cross symbol represents minimum curvature.}
  \label{fig:apd_curs}
\end{figure}

As shown in Figure~\ref{fig:apd_curs}, the average curvature is still larger than the minimum curvature (especially when the regularization term is small). Despite this, the average curvature of KDDCup99 is smaller than Adult, this may be the reason why the improvement in Section~\ref{sec:exp} is larger for the Adult dataset.

 \end{appendices}
